# Supplementary material for: Orbital Selective Superconductivity in a Two-band Model of Infinite-Layer Nickelates
Source: arXiv:2005.01243 source file (2020-05-04)
Supplement: Supplementary file 1 [file supplemental.pdf]

# Supplemental Material:Orbital Selective Superconductivity in Two-band Model of Infinite-Layer Nickelates


Priyo Adhikary* and Tanmoy Das*
*Department of Physics, Indian Institute of Science, Bangalore 560012, India.*

Subhadeep Bandyopadhyay* and Indra Dasgupta†
*School of Physical Sciences, Indian Association for the Cultivation of Science, Kolkata 700 032, India.*

Tanusri Saha-Dasgupta‡
*S. N. Bose National Centre for Basic Sciences, JD Block,*
*Sector III, Salt Lake, Kolkata, West Bengal 700106, India.*

## DFT COMPUTATIONAL DETAILS

The first principles electronic structure calculations have been performed within the framework of density functional theory (DFT) using the plane-wave basis with projector augmented wave (PAW)[1] potential as implemented in the Vienna Abinitio Simulation Package (VASP) [2]. Generalized gradient approximation (GGA) implemented within Perdew-Burke-Ernzerhof (PBE)[3] prescription has been chosen as the exchange-correlation functional. A plane wave cut-off of 600 eV was set to get good convergence of total energy and a k-mesh of $16 \times 16 \times 16$ was used for the Brilliouin zone integration. The energy convergence criterion was set to $10^{-6}$ eV during the energy minimization process of the self-consistent cycle. Maximally localized Wannier functions (MLWFs) for the low energy two band model have been constructed using the formulation of WANNIER90 [4].

## HOPPING PARAMETERS FOR THE TWO BAND MODEL

TABLE I. Hopping parameters for the two band model for $NdNiO_2$

| i | j | k | $t^{s-s}{}_{[i,j,k]}$ (eV) |
|---|---|---|---|
| 0 | 0 | 0 | 1.398 |
| 0 | 0 | 1 | -0.171 |
| 1 | 0 | 0 | -0.029 |
| 1 | 0 | 1 | -0.218 |
| 1 | 1 | 0 | -0.093 |
| 1 | 1 | 1 | 0.066 |
| 0 | 0 | 2 | -0.209 |
| 1 | 0 | 2 | 0.042 |
| 0 | 2 | 0 | 0.022 |
| i | j | k | $t^{d-d}{}_{[i,j,k]}$ (eV) |
| 0 | 0 | 0 | 0.273 |
| 0 | 0 | 1 | -0.037 |
| 1 | 0 | 0 | -0.368 |
| 1 | 0 | 1 | -0.002 |
| 1 | 1 | 0 | 0.082 |
| 1 | 1 | 1 | 0.013 |
| 0 | 0 | 2 | 0.003 |
| 1 | 0 | 2 | 0.001 |
| 0 | 2 | 0 | -0.042 |
| i | j | k | $t^{s-d}{}_{[i,j,k]}$ (eV) |
| 0 | 0 | 1 | 0.001 |
| 1 | 0 | 0 | 0.071 |
| 1 | 0 | 1 | 0.001 |
| 1 | 1 | 0 | 0.001 |
| 1 | 1 | 1 | 0.001 |
| 0 | 0 | 2 | 0.000 |
| 1 | 0 | 2 | 0.031 |
| 0 | 2 | 0 | 0.008 |

TABLE II. Hopping parameters for the two band model for $LaNiO_2$

| i | j | k | $t^{s-s}{}_{[i,j,k]}$ (eV) |
|---|---|---|---|
| 0 | 0 | 0 | 1.153 |
| 0 | 0 | 1 | -0.026 |
| 1 | 0 | 0 | -0.024 |
| 1 | 0 | 1 | -0.166 |
| 1 | 1 | 0 | -0.066 |
| 1 | 1 | 1 | 0.026 |
| 0 | 0 | 2 | -0.115 |
| 1 | 0 | 2 | 0.035 |
| 0 | 2 | 0 | -0.001 |
| i | j | k | $t^{d-d}{}_{[i,j,k]}$ (eV) |
| 0 | 0 | 0 | 0.260 |
| 0 | 0 | 1 | -0.032 |
| 1 | 0 | 0 | -0.345 |
| 1 | 0 | 1 | -0.001 |
| 1 | 1 | 0 | 0.088 |
| 1 | 1 | 1 | 0.009 |
| 0 | 0 | 2 | 0.006 |
| 1 | 0 | 2 | 0.000 |
| 0 | 2 | 0 | -0.033 |
| i | j | k | $t^{s-d}{}_{[i,j,k]}$ (eV) |
| 0 | 0 | 1 | -0.003 |
| 1 | 0 | 0 | 0.059 |
| 1 | 0 | 1 | -0.004 |
| 1 | 1 | 0 | 0.001 |
| 1 | 1 | 1 | -0.002 |
| 0 | 0 | 2 | 0.002 |
| 1 | 0 | 2 | 0.018 |
| 0 | 2 | 0 | 0.013 |

Hopping parameters for the two band model are given in Table.I and Table.II for $NdNiO_2$ and $LaNiO_2$ respectively. Here axial and Ni-$d_{x^2-y^2}$ orbitals are represented as $s$ and $d$ respectively. $t^{s-s}$, $t^{d-d}$ and $t^{s-d}$ represents the hopping between axial-axial, Ni-$d_{x^2-y^2}$-Ni-$d_{x^2-y^2}$ and axial-Ni-$d_{x^2-y^2}$ orbitals respectively as function of integers i, j, k. The integers i, j, k represents hopping between the unit cells in the respective directions with a relative distance $\vec{r}$ =i$\vec{a}$ + j$\vec{b}$ + k$\vec{c}$, where $\vec{a}$, $\vec{b}$, $\vec{c}$ are the unit cell vectors. i = j = k = 0 represents the onsite energy. Fermi energy is set at 0 eV for both the systems.

## SUPERCONDUCTIVITY

For the interaction, we consider a two band Hubbard model,

$$H' = \sum_{\alpha\in s,d} \sum_{\mathbf{k},\mathbf{k}',\mathbf{q}} U_\alpha c^\dagger_{\alpha\uparrow}(\mathbf{k}) c^\dagger_{\alpha\downarrow}(\mathbf{k}') c_{\alpha\downarrow}(\mathbf{k}'-\mathbf{q}) c_{\alpha\uparrow}(\mathbf{k}+\mathbf{q})$$
$$+ \sum_{\sigma=\uparrow,\downarrow} \sum_{\mathbf{k},\mathbf{k}',\mathbf{q}} V_{ds} c^\dagger_{d\sigma}(\mathbf{k}) c^\dagger_{s,\sigma'}(\mathbf{k}') c_{s,\sigma'}(\mathbf{k}'-\mathbf{q}) c_{d\sigma}(\mathbf{k}+\mathbf{q}). \quad (1)$$

$U_d$, and $U_s$ are the intra-orbital Hubbard interaction, while $V_{ds}$ gives the intra-orbital one (local). $c^{\dagger}_{\alpha,\sigma}(\mathbf{k})$ gives the creation operator for the $\alpha$-orbital with spin $\sigma =\uparrow / \downarrow$ at the wavevector $\mathbf{k}$. By expanding the interaction term to multiple interaction channels, and collecting the terms which give a pairing interaction (both singlet and triplet channels are considered) we obtain the effective pairing potential $\Gamma^{\gamma\delta}_{\alpha\beta}(\mathbf{q})$ as[5–8]

$$H_{\rm int} \approx \frac{1}{\Omega^2_{\rm BZ}} \sum_{\alpha\beta\gamma\delta} \sum_{\mathbf{kq},\sigma\sigma'} \Gamma^{\gamma\delta}_{\alpha\beta}(\mathbf{q}) \times c^{\dagger}_{\alpha\sigma}(\mathbf{k}) c^{\dagger}_{\beta\sigma'}(-\mathbf{k}) c_{\gamma\sigma'}(-\mathbf{k}-\mathbf{q}) c_{\delta\sigma}(\mathbf{k}+\mathbf{q}). \tag{2}$$

$\sigma' = \pm\sigma$ give triplet and singlet pairing channels, respectively. This pairing potential, obtained in Refs. [5], includes a summation of bubble and ladder diagrams within the random phase approximation (RPA). The pairing potential in general involves four orbital indices and thus is a tensor in the orbital basis. We denote all such tensors by the 'tilde' symbol. The pairing potentials in the singlet ($\tilde{\Gamma}_{\uparrow\downarrow}$) and triplet ($\tilde{\Gamma}_{\uparrow\uparrow}$) channels are

$$\tilde{\Gamma}_{\uparrow\downarrow}(\mathbf{q}) = \frac{1}{2}\big[3\tilde{U}_s\tilde{\chi}_s(\mathbf{q})\tilde{U}_s - \tilde{U}_c\tilde{\chi}_c(\mathbf{q})\tilde{U}_c + \tilde{U}_s + \tilde{U}_c\big], \tag{3a}$$

$$\tilde{\Gamma}_{\uparrow\uparrow}(\mathbf{q}) = -\frac{1}{2}\big[\tilde{U}_s\tilde{\chi}_s(\mathbf{q})\tilde{U}_s + \tilde{U}_c\tilde{\chi}_c(\mathbf{q})\tilde{U}_c - \tilde{U}^s - \tilde{U}_c\big]. \tag{3b}$$

Here subscript 's' and 'c' denote spin and charge fluctuation channels, respectively. $\tilde{U}_{s/c}$ are the onsite interaction tensors for spin and charge fluctuations, respectively, defined in the same basis as $\tilde{\Gamma}$. Its non-vanishing components are given in the main text.

$\tilde{\chi}_{s/c}$ are the density-density correlators (tensors in the same orbital basis) for the spin and charge density channels. We define the non-interacting density-density correlation function (Lindhard susceptibility) $\tilde{\chi}_0$ within the standard linear response theory:

$$[\chi_0(\mathbf{q})]^{\gamma\delta}_{\alpha\beta} = -\frac{1}{\Omega_{\rm BZ}} \sum_{\mathbf{k},\nu\nu'} \phi^{\nu}_{\beta}(\mathbf{k})\phi^{\nu *}_{\alpha}(\mathbf{k})\phi^{\nu'}_{\delta}(\mathbf{k}+\mathbf{q})\phi^{\nu' *}_{\gamma}(\mathbf{k}+\mathbf{q}) \times \frac{f(E_{\nu'}(\mathbf{k}+\mathbf{q})) - f(E_{\nu}(\mathbf{k}))}{E_{\nu'}(\mathbf{k}+\mathbf{q}) - E_{\nu}(\mathbf{k}) + i\epsilon}. \tag{4}$$

$E_{\nu}(\mathbf{k})$ are the eivenvalues of the two Wannier orbital Hamiltonians and $\phi^{\nu}_{\alpha}(\mathbf{k})$ gives a component of the eigenvector. $f$ is the Fermi distributions function. Many body effect of Coulomb interaction in the density-density correlation is captured within $S$-matrix expansion of Hubbard Hamiltonian in Eq. (1). By summing over different bubble and ladder diagrams we obtain the RPA spin and charge susceptibilities as:

$$\tilde{\chi}_{\rm s/c}(\mathbf{q}) = \tilde{\chi}_0(\mathbf{q}) \left(\tilde{\mathbb{I}} \mp \tilde{U}_{s/c}\tilde{\chi}_0(\mathbf{q})\right)^{-1}, \tag{5}$$

where $\tilde{\mathbb{I}}$ is the unit matrix.

Eq. (2) gives the pairing interaction for pairing between orbitals. However, we solve the BCS gap equation in the band basis. To make this transformation, we make use of the unitary transformation $c_{\alpha\sigma} \to \sum_{\nu} \mathcal{U}^{\alpha}_{\nu}\gamma_{\nu\sigma}$ for all $\mathbf{k}$ and spin $\sigma$. With this substitution we obtain the pairing interaction Hamiltonian in the band basis as

$$H_{\rm int} \approx \sum_{\nu\nu'} \sum_{\mathbf{kq},\sigma\sigma'} \Gamma'_{\nu\nu'}(\mathbf{k},\mathbf{q}) \times \frac{1}{\Omega^2_{\rm BZ}} \gamma^{\dagger}_{\nu\sigma}(\mathbf{k})\gamma^{\dagger}_{\nu\sigma'}(-\mathbf{k})\gamma_{\nu'\sigma'}(-\mathbf{k}-\mathbf{q})\gamma_{\nu'\sigma}(\mathbf{k}+\mathbf{q}). \tag{6}$$

The same equation holds for both singlet and triplet pairing and thus henceforth we drop the corresponding symbol for simplicity. The band pairing interaction $\Gamma'_{\nu\nu'}$ is related to the corresponding orbital one as $\Gamma'_{\nu\nu'}(\mathbf{k},\mathbf{q}) = \sum_{\alpha\beta\gamma\delta} \Gamma^{\gamma\delta}_{\alpha\beta}(\mathbf{q})\phi^{\nu\dagger}_{\alpha}(\mathbf{k})\phi^{\nu\dagger}_{\beta}(-\mathbf{k})\phi^{\nu'}_{\gamma}(-\mathbf{k}-\mathbf{q})\phi^{\nu'}_{\delta}(\mathbf{k}+\mathbf{q})$. We define the SC gap in the $\nu^{\rm th}$-band as

$$\Delta_{\nu}(\mathbf{k}) = -\frac{1}{\Omega_{\rm BZ}} \sum_{\nu',\mathbf{q}} \Gamma'_{\nu\nu'}(\mathbf{k},\mathbf{q}) \left\langle \gamma_{\nu'\sigma'}(-\mathbf{k}-\mathbf{q})\gamma_{\nu'\sigma}(\mathbf{k}+\mathbf{q})\right\rangle, \tag{7}$$

where the expectation value is taken over the BCS ground state. In the limit $T \to 0$ we have $\langle \gamma_{\nu\sigma}(-\mathbf{k})\gamma_{\nu\sigma}(\mathbf{k})\rangle \to \lambda\Delta_\nu(\mathbf{k})$, with $\lambda$ is the SC coupling constant. Substituting this in Eq. (7), we get

$$\Delta_\nu(\mathbf{k}) = -\lambda\frac{1}{\Omega_{\rm BZ}}\sum_{\nu',\mathbf{q}}\Gamma'_{\nu\nu'}(\mathbf{k},\mathbf{q})\Delta_{\nu'}(\mathbf{k}+\mathbf{q}). \quad (8)$$

This is an eigenvalue equation of the pairing potential $\Gamma'_{\nu\nu'}(\mathbf{q}=\mathbf{k}-\mathbf{k}')$ with eigenvalue $\lambda$ and eigenfunction $\Delta_\nu(\mathbf{k})$. The $\mathbf{k}$-dependence of $\Delta_\nu(\mathbf{k})$ dictates the pairing symmetry for a given eigenvalue. While there are many solutions (as many as the $\mathbf{k}$-grid), however, we consider the highest eigenvalue since this pairing symmetry can be shown to have the lowest Free energy value in the SC state.[5]

* tnmydas@gmail.com
† sspid@iacs.res.in
‡ t.sahadasgupta@gmail.com

[1] G. Kresse and D. Joubert, Phys. Rev. B **59**, 1758 (1999).
[2] G. Kresse et.al., Phys. Rev. B **54**, 11169 (1996).
[3] J. P. Perdew, K. Burke and M. Ernzerhof, Phys. Rev. Lett. **77**, 3865 (1996).
[4] A. A. Mostofi, J. R. Yates, Y.-S. Lee, I. Souza, D. Vanderbilt and N. Marzari Comput. Phys. Commun. **178**, 685 (2008).
[5] D. J. Scalapino, Rev. Mod. Phys. **84**, 1383 (2012); A. V. Chubukov, D. Pines, J. Schmalian, In: Bennemann K.H., Ketterson J.B. (eds) The Physics of Superconductors. Springer, Berlin, Heidelberg; T Das, RS Markiewicz, A Bansil, Adv. Phys. **63**, 151 (2014).
[6] D. J. Scalapino, E. Loh, Jr., and J. E. Hirsch, Phys. Rev. B **34**, 8190 (R) (1986); *ibid* Phys. Rev. B **34**, 6420 (1986); J. R. Schrieffer, *Theory of Superconductivity* (W. A. Benjamin, New York) (1964); J. R. Schrieffer, X. G. Wen, and S. C. Zhang, Phys. Rev. B **39**, 11663 (1989); P. Monthoux, A. V. Balatsky, and D. Pines, Phys. Rev. Lett. **67**, 3448 (1991); M. Sigrist, and Kazuo Ueda, Rev. Mod. Phys. **63**, 239 (1991); D. J. Scalapino, Rev. Mod. Phys. **84**, 1383 (2012); J. C. Seamus Davis and Dung-Hai Lee, PNAS **110**, 17623-17630 (2013); T Das, RS Markiewicz, A Bansil, Adv. Phys. **63**, 151 (2014).
[7] I. I. Mazin, D. J. Singh, M. D. Johannes, and M. H. Du, Phys. Rev. Lett. **101**, 057003S (2008); S. Graser, T. A. Maier, P. J. Hirschfeld, D. J. Scalapino, New J. Phys. **11**, 025016 (2009); Zi-Jian Yao, Jian-Xin Li, and Z D Wang, New J. Phys. **11**, 025009 (2009); T. Das, A. V. Balatsky, Phys. Rev. B **84**, 014521 (2011); A. Chubukov, Ann. Rev. Conden. Mat. Phys. **3**, 57-92 (2012).
[8] Tetsuya Takimoto, Takashi Hotta, and Kazuo Ueda, Phys. Rev. B **69**, 104504 (2004); K. Kubo, Phys. Rev. B **69**, 104504 (2004); T. Das, J.-X. Zhu, M. J. Graf, Sci. Rep. **5,** 8632 (2015); Hiroaki Ikeda, Michi-To Suzuki, Ryotaro Arita, Phys. Rev. Lett. **114**, 147003 (2015); T. Nomoto, H. Ikeda, Phys. Rev. Lett. **117**, 217002 (2016); T. Nomoto, H. Ikeda, J. Phys. Soc. Jpn. **86**, 023703 (2017).
